# Supplementary material for: ObPose: Leveraging Pose for Object-Centric Scene Inference and Generation in 3D
Source: arXiv:2206.03591 source file (2023-06-09)
Supplement: Supplementary file 1 [file 6_appendix.tex]

\section{Appendix}
\label{sec:appendix}
\subsection{Minimum Volume Principle in Detail}
The proposed approach for recovering the pose of an object is described in Algorithm \ref{alg:min_vol}. A visualisation of how the estimated pose evolves as the volume of the AABB that contains the object decreases is depicted in \Cref{fig:min_volume}. An advantage of the proposed minimum volume principle is that the recovered pose will align one of its coordinate planes with the symmetry plane of the object if it exists.
\begin{figure*}[ht]
    \centering
    \includegraphics[width=1.0\linewidth]{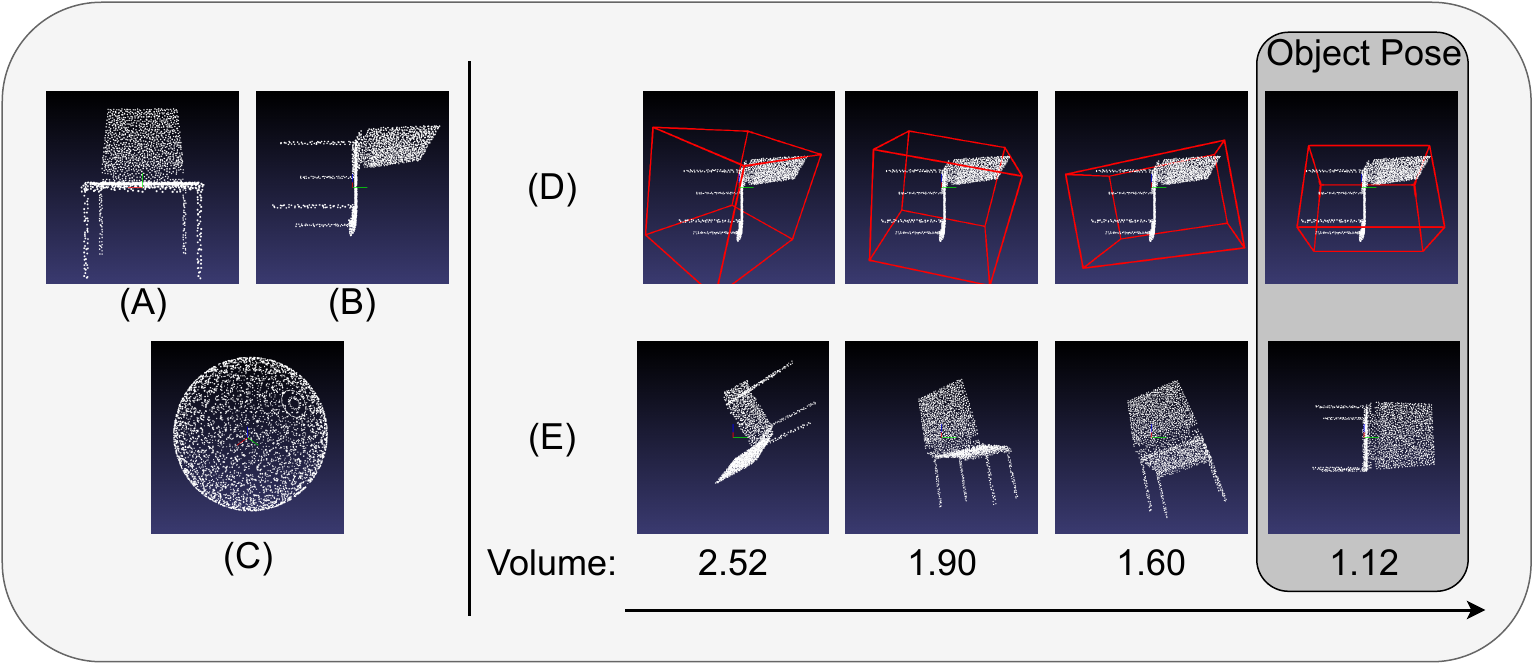}
    \vspace{-0.1cm}
    \caption{We demonstrate the point cloud of a chair (A) in arbitrary pose (B) and how its pose is recovered using the minimum volume principle. The selection matrices $\mathbf{R}^{s}$ are illustrated in (C) by rotating a point at $[1,1,1]$ with all the selection matrices. (D) and (E) depict how the estimated object orientation represented by a bounding box and the object viewed with respect to its reference pose evolve with respect to the volume of the AABB. }
    \label{fig:min_volume}
\end{figure*}
\input{supp_pseudocode}
\subsection{Training and Implementation Details}
\label{imp_details}
Training takes about 35 hours for the YCB moving-object dataset and 20 hours for the YCB static dataset on a single NVIDIA Titan RTX GPU. The video model and the static model are trained for 100k and 100.5k iterations, each with a batch size of 2 and 8, respectively, selected according to the available GPU memory. The IC-SBP ablation has a batch size of 8 for the video experiments as it's a static image-based approach. 
%For ObSuRF, we train for 90k and 100.5k with a batch size of 32 for the video and static image data. 
Video length is 5 frames randomly cropped from the full video for training and we use the full video length (typically 15 frames or longer) for testing. The model is thus able to process videos that are much longer than the videos seen during training. The YCB moving-object dataset has 4000 videos for training and 500 videos for testing. The YCB static dataset has 12000 scenes for training and 1500 scenes for testing. We summarise all the hyper-parameters in \Cref{table:hyper}. In the ablation study we use slot attention with a background slot as introduced in \citet{yu2021unsupervised}. For video data, slots from the last time step are used to initialise slot attention at the current time step. For both datasets, \obpose~ estimates poses with all points below the ground surface being neglected, as we find that NeRF can mistakenly predict the occupancy of the points below the ground surface whose x-y coordinates are within the object's convex hull. This (erroneous) generalisation follows from the fact that this part of the scene receives no training signal, due to the ray marching used in NeRFs.
For the training on the CLEVR dataset, we find that using a L2 loss rather than a mixture of Gaussian loss for the \cref{attention_mask} can improve the robustness of the training, i.e.:
\begin{equation}
    \mathcal{L}_{\text{att}}= \sum_{k=1}^{K} (\mathcal{N}(\mathbf{x}|\mathbf{c}_{k},\sigma_{\text{std}}^{2})/\mathcal{N}(0|0,\sigma_{\text{std}}^{2}) - \mathbf{m}_{k})^{2} + \sum_{k=1}^{K} (\mathbf{m}_{k} - \hat{\mathbf{\sigma}}^{\text{surface}}_{k}/\sigma_{\text{max}})^{2}
\end{equation}
\subsection{Network Structures}
The KPConv encoder backbone consists of an input block and three consecutive encoding blocks with radiuses of $[0.025,0.05,0.1,0.2 ]$ meters for the KPConv layers. Each block has three sub-blocks which each has a structure of \textit{Conv1d-Group norm\citep{wu2018group}-ReLU-KPConv-Conv1d-Group norm-ReLU} with a skip connection being built between the output of the first ReLU layer and the output. The skip connection takes the output of the ReLU and feeds it into a Conv1d layer followed by a Group norm. The input block consists of an input layer of \textit{KPConv-Group norm-ReLU} and a single sub-block as described above. For the input block and all the sub-blocks, the number of channels are $[16,16,32,32,32,64,64,64,64,64,64]$ respectively and the strides are $[8,1,4,1,1,4,1,1,4,1,1]$. The KPConv-aggregate layer has a channel number of $64$ and a radius of $1$ meter. Two trilinear interpolation layers are used to up-sample the embedding and predict embedding of $64$ channels and $32$ channels respectively. A \textit{Conv1d-Group norm-ReLU} encoding is used in both the input and the skip connection between the input and the output of the interpolation layer. A final output layer of structure \textit{Conv1d-Group norm-LeakyReLU(0.1)-Conv1d} is appended to the output embedding with channel numbers of $32$ and $16$ for the two Conv1d layers.
The \textit{where} encoder and the \textit{what} encoder share the same structure of the backbone encoder and have channel numbers of $[16,16,32,32,32,64,64,64,64,64,64]$ and strides of $[1,1,4,1,1,4,1,1,4,1,1]$. A final output layer of structure \textit{Linear-Group norm-LeakyReLU(0.1)-Linear} is used to predict the final embedding. Both linear layers have $64$ output channels.
The RNNs used to parameterise the posterior and the prior distribution of the \textit{where} and the \textit{what} latent embedding has a dimension of $32$ for the hidden state followed by an MLP of size $[32,32,64]$ with the output $64$ channels being further divided into the mean and the standard deviation of the Gaussian. The $\mathbf{z}^{\text{\textit{where}}}$ is decoded into the $\Delta \mathbf{T}$ using an MLP of sizes $[32,256,3]$.   
We use the default NeRF decoder open-sourced by \citet{niemeyer2021giraffe}. 
%Our code is available at: https://github.com/ObPose/ObPose.

\begin{table*}[ht]
    \centering
    \caption{Hyperparameters of \obpose. }
    \label{table:hyper}
    \begin{adjustbox}{max width=1.0\textwidth}
    \begin{tabular}{l l r}
        \hline
        Parameter & Description & Value\\
        $\mathbf{\sigma}_{\text{std}}$ & Standard deviation of colour dist. & 0.1 \\
        $\mathbf{\sigma}_{\text{max}}$ & Maximum density & 10/1 for YCB/CLEVR \\
        $s$ & Bounding box size & 0.4/0.2 for YCB/CLEVR \\
        $N_{\text{thresh}}$ & Number of points to use the pose of last time step & 10 \\
        $T_{\text{max}}$ & Maximally allowed $\Delta \mathbf{T}$ & 0.1 \\
        $\mathbf{S}$ & Number of sparse voxels along each dimension & 24 \\
        $\delta$ & Noise added to depths $d_{\text{surface}}$ & 0.01/0.7 for YCB/CLEVR \\
        $\beta$ & tolerance factor to select minimum volume bounding box & 0.1/0.01 for video/static images \\
        $K$ & Number of slots for IC-SBP & 4 \\
        $d_{z}^{what}$ & Dimensionality of $\mathbf{z}^{\text{\textit{what}}}$   & 32/256 for YCB/CLEVR \\
        $d_{z}^{where}$ & Dimensionality of
        $\mathbf{z}^{\text{\textit{where}}}$ & 32
        \\
        \bottomrule
    \end{tabular}
    \end{adjustbox}
\end{table*}
\subsection{Segmentation Results on YCB Static}
We illustrate additional segmentation results on YCB static dataset in \Cref{fig:seg_static}.
\begin{figure*}[h]
    \centering
    \includegraphics[width=1.0\linewidth]{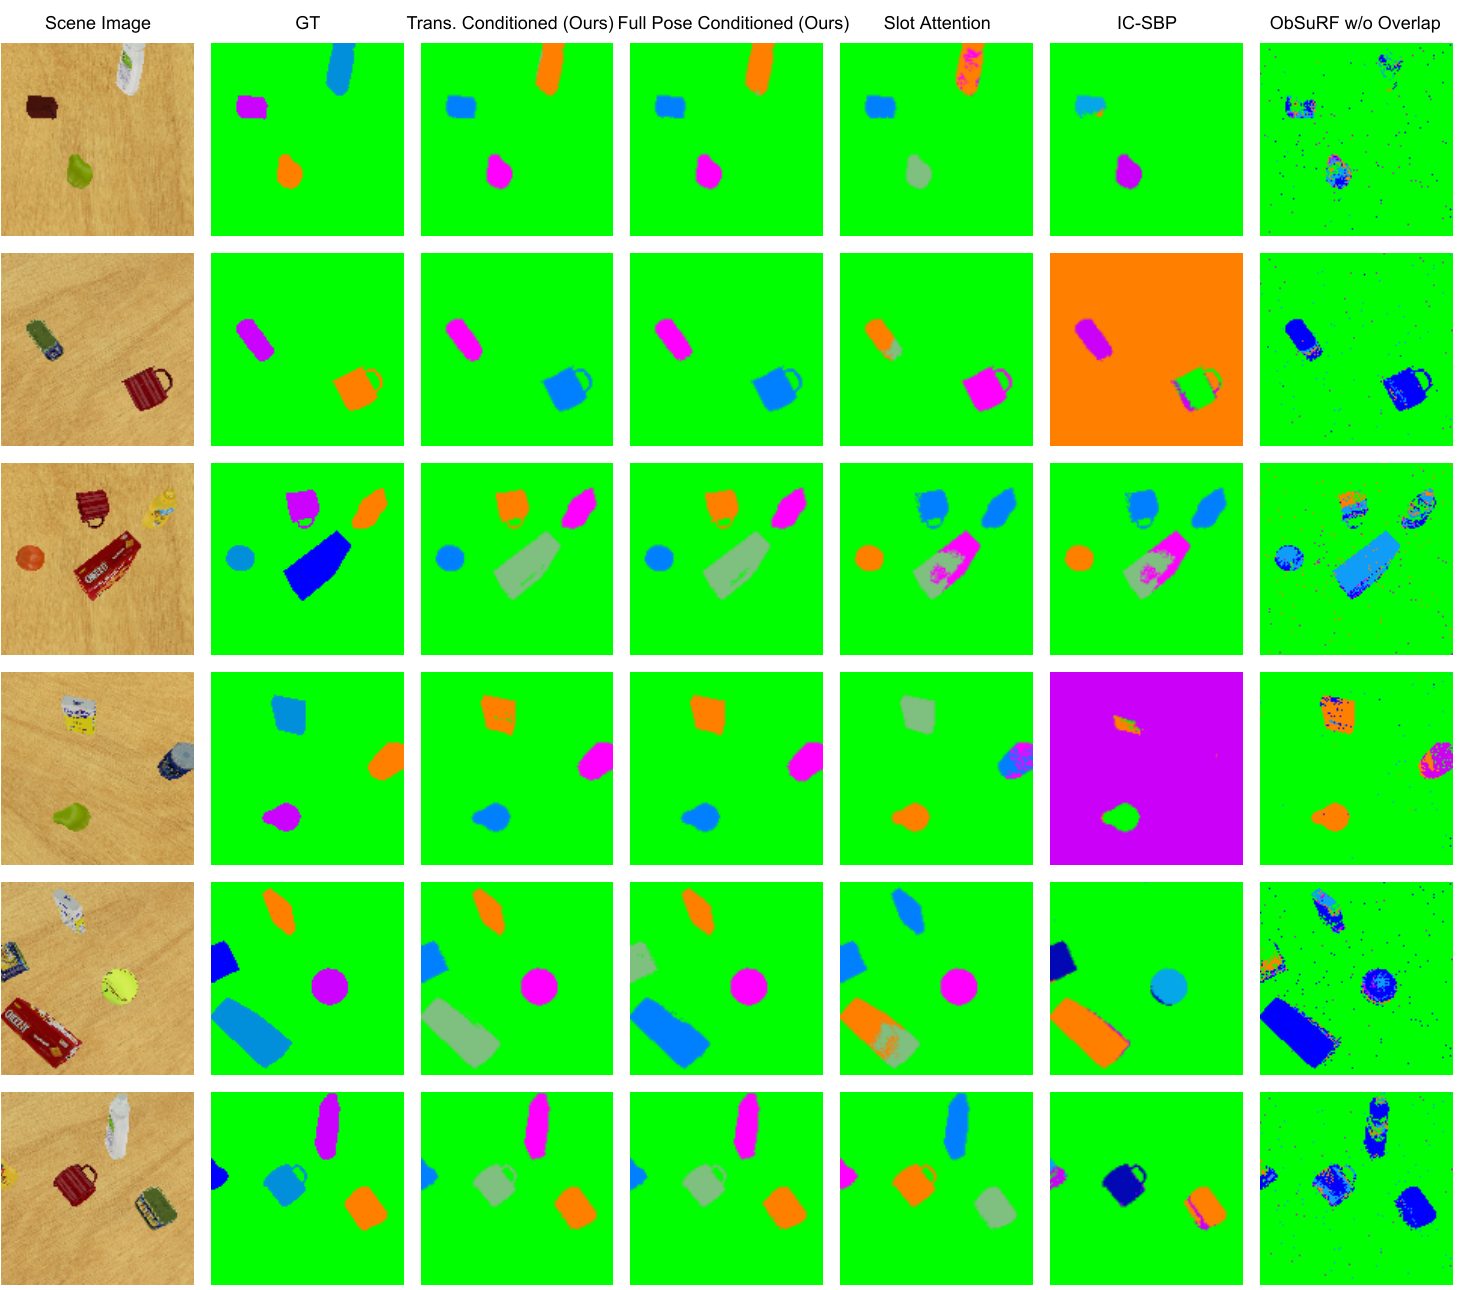}
    \vspace{-0.1cm}
    \caption{Qualitative results on YCB static dataset. }
    \label{fig:seg_static}
\end{figure*}
\subsection{Rendering Results on YCB Static}
We illustrate additional NeRF rendering results on YCB static dataset in \Cref{fig:render_static}.
\begin{figure*}[h]
    \centering
    \includegraphics[width=1.0\linewidth]{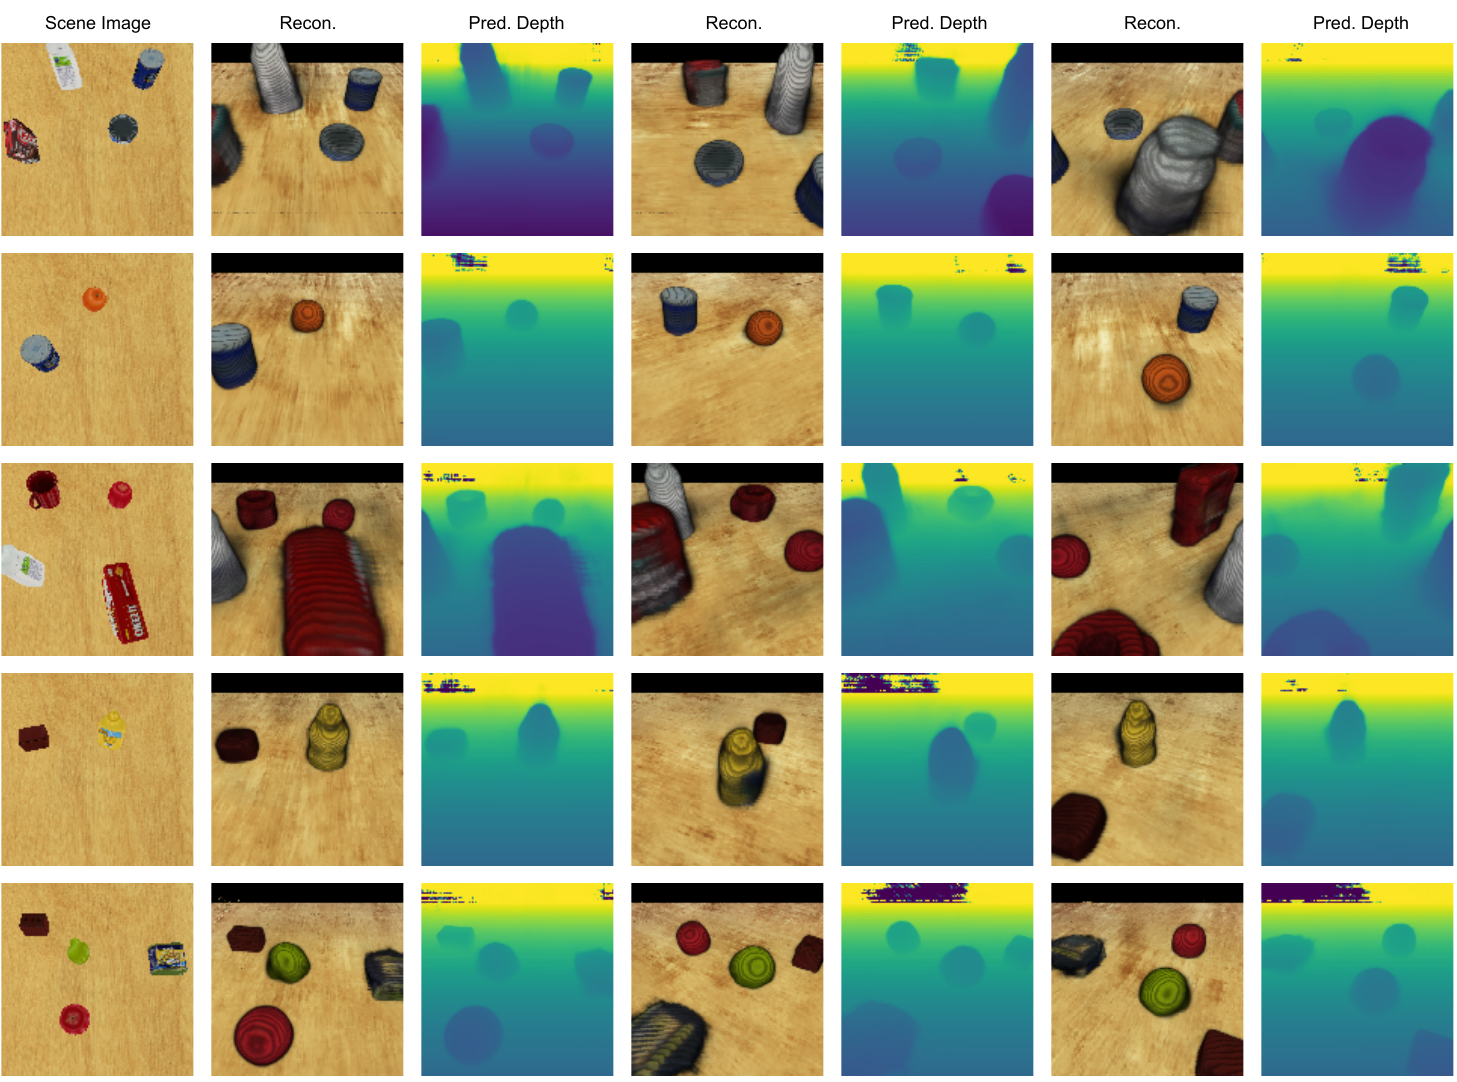}
    \vspace{-0.1cm}
    \caption{NeRF rendering results on YCB static dataset. }
    \label{fig:render_static}
\end{figure*}
\subsection{Results on CLEVR-3D}
We show qualitative results on CLEVR-3D dataset in \Cref{fig:seg_clevr}. We find that \obpose~can segment part of the shadows of the objects as part of the objects because the shadows are caused by the existence of the objects. The shape of the objects can be recovered even \obpose~is trained without multi-view supervisions.
\begin{figure*}[ht]
    \centering
    \includegraphics[width=1.0\linewidth]{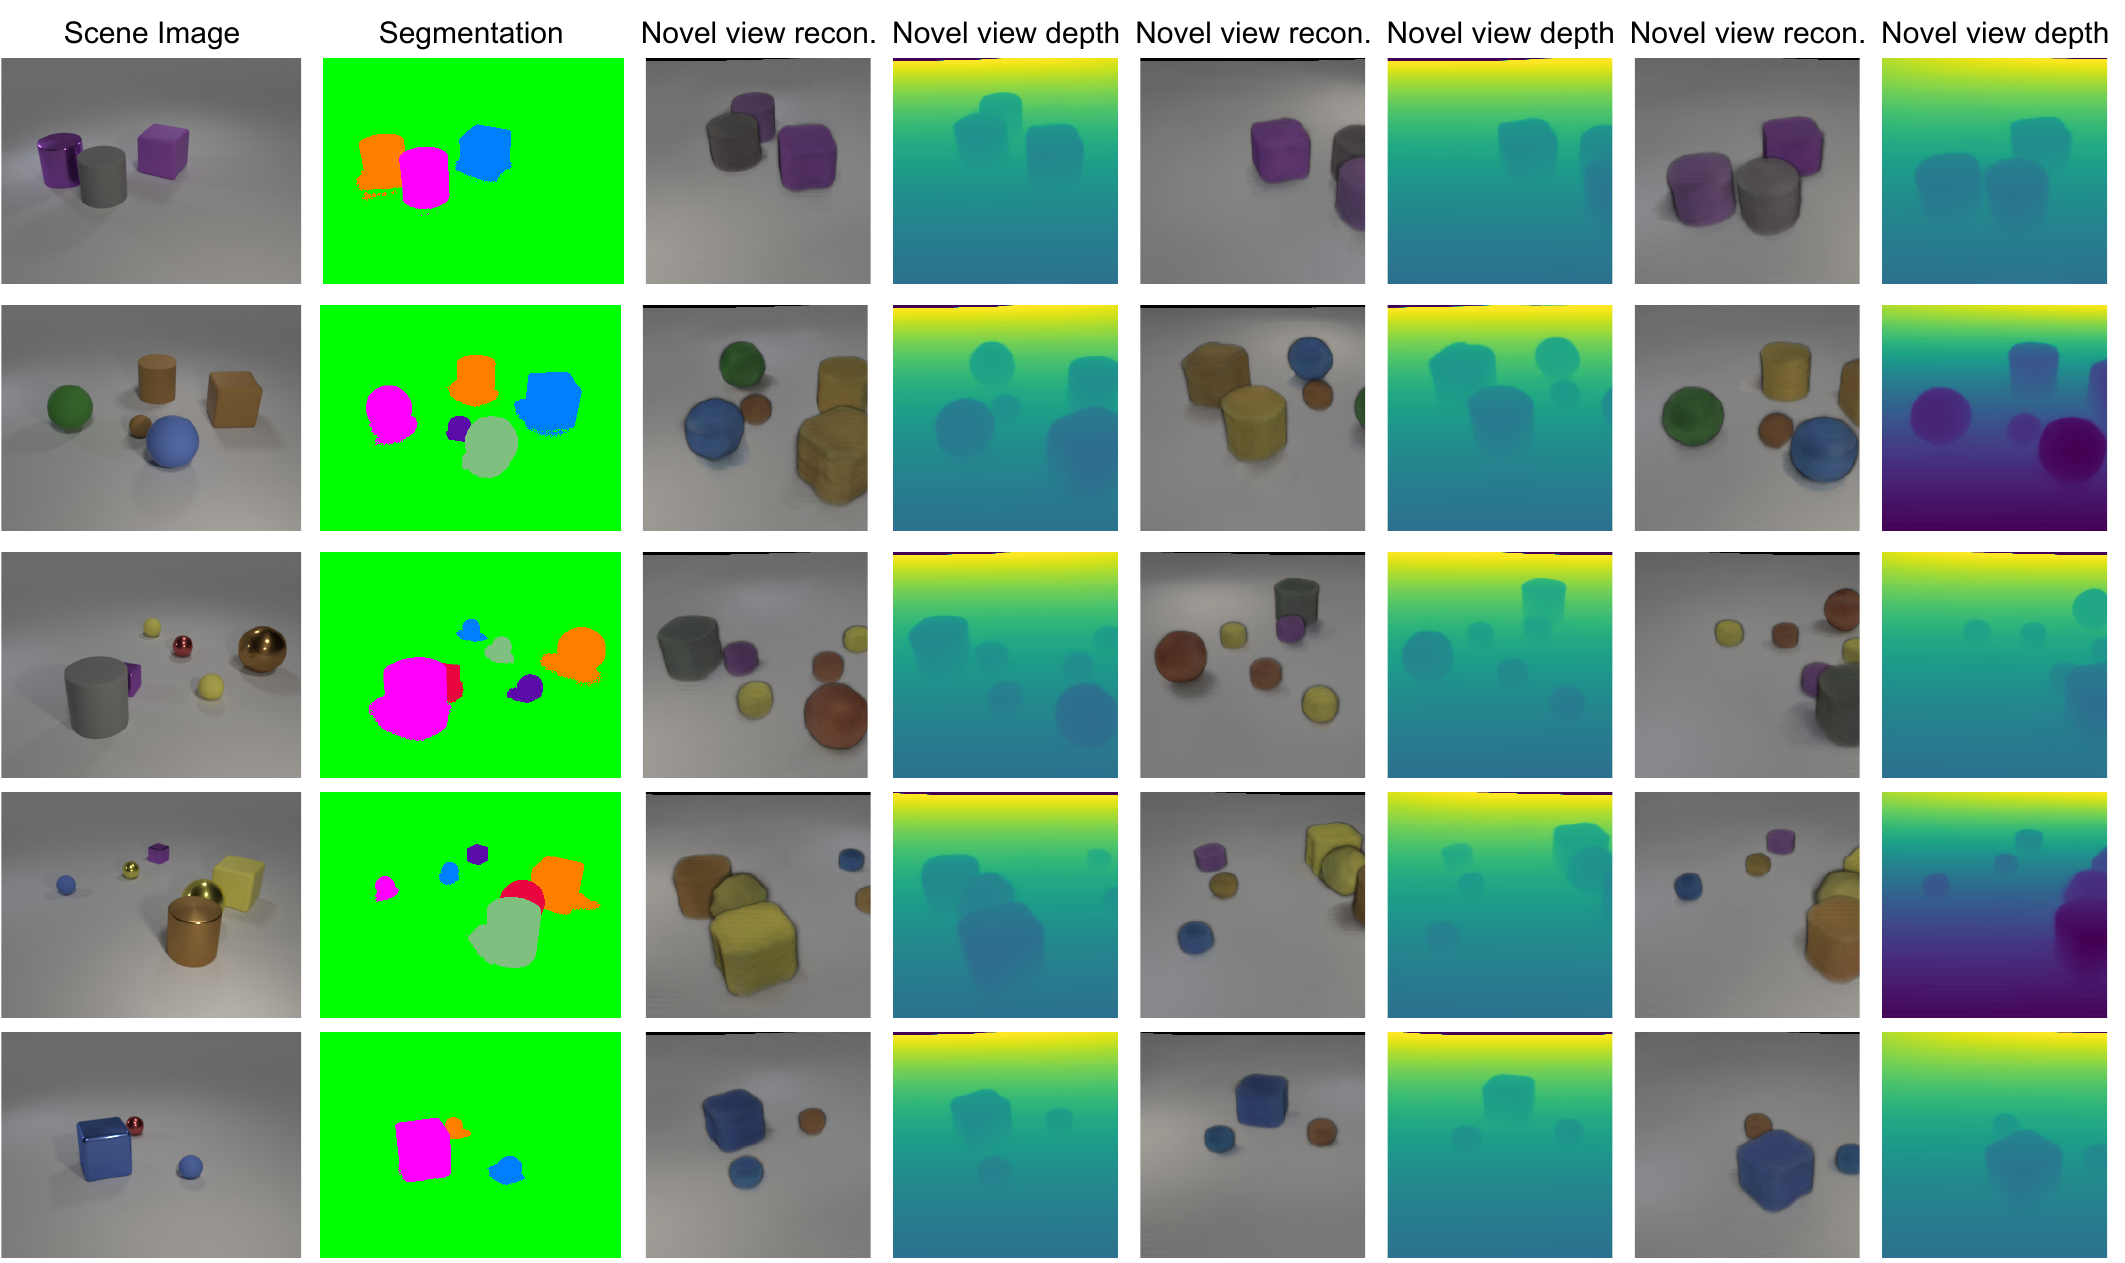}
    \vspace{-0.1cm}
    \caption{Qualitative results on CLEVR-3D dataset. }
    \label{fig:seg_clevr}
\end{figure*}
\subsection{Comparison between Video Inputs and Single Frame Inputs}
We show \obpose's~performence taking video inputs and single frame inputs in \Cref{table:segmentation_single_video} and \Cref{fig:seg_single_video} respectively. We find that \obpose's~performance is only slightly worse with single frame inputs, but the ability of tracking objects is lost in that input setting.
\begin{figure*}[ht]
    \centering
    \includegraphics[width=1.0\linewidth]{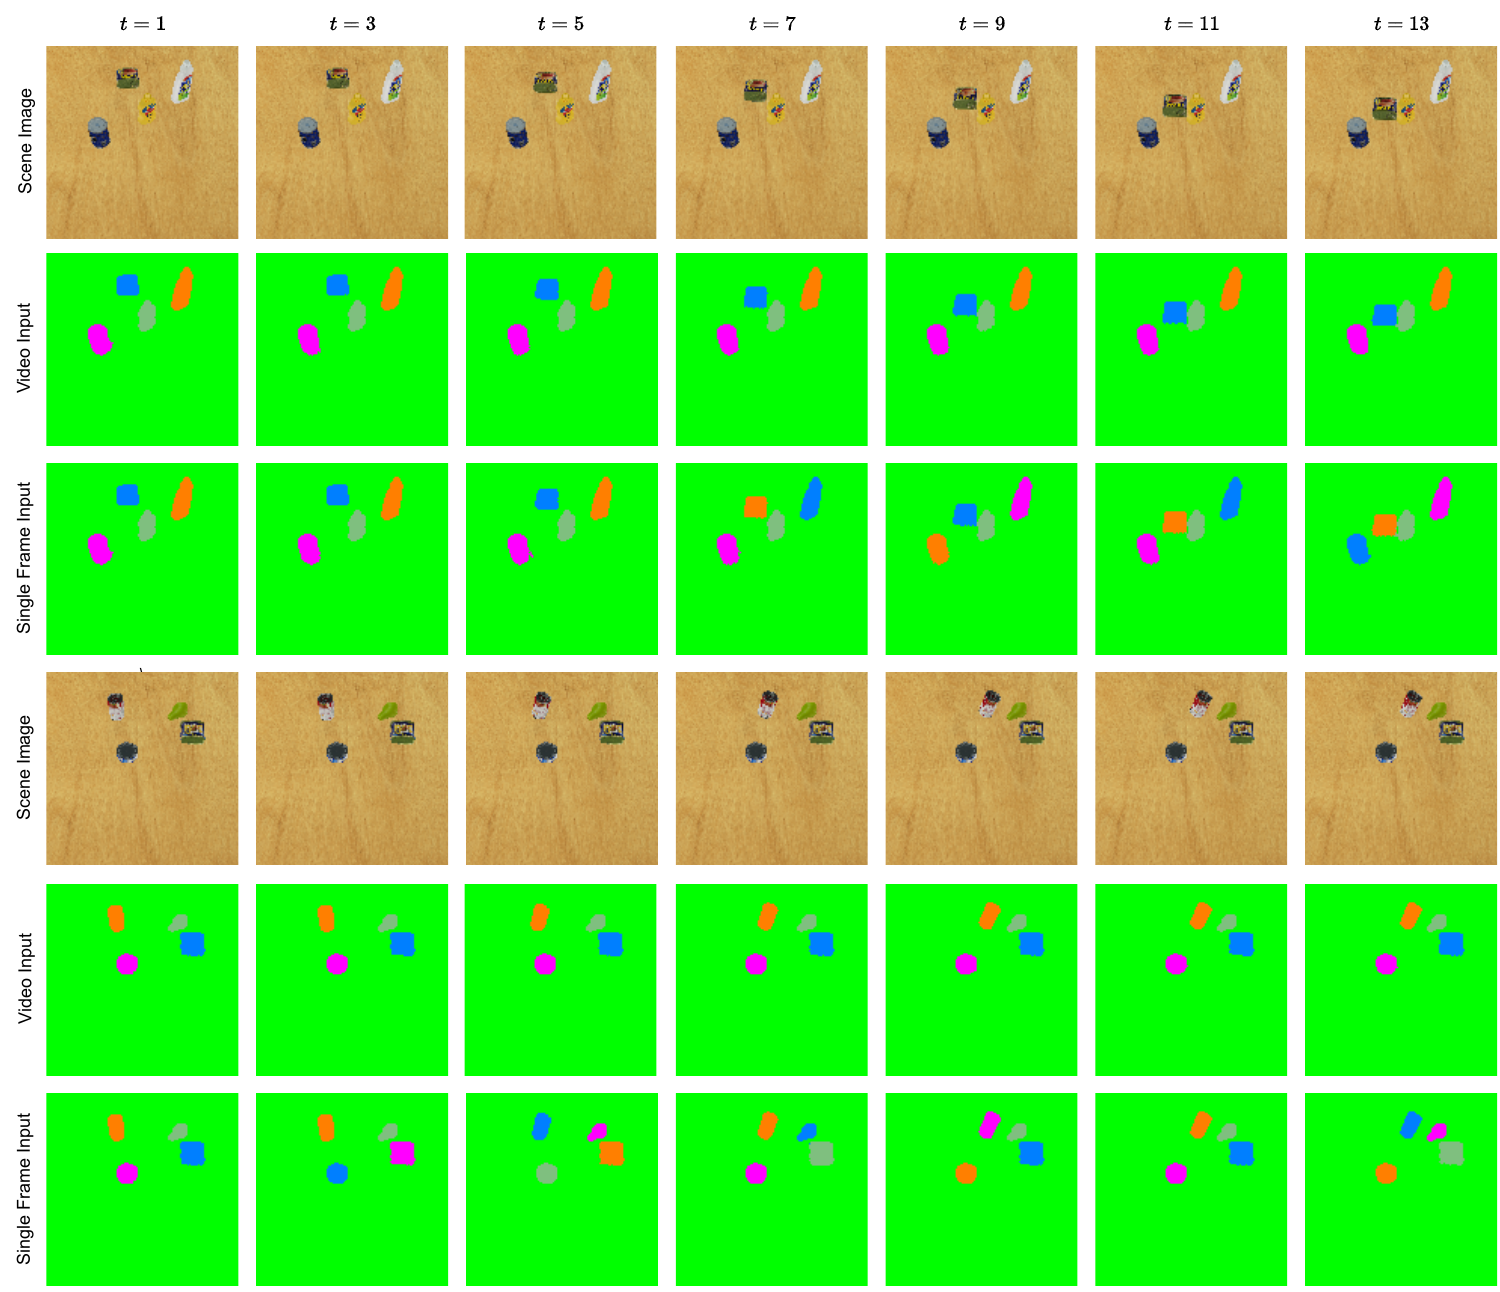}
    \vspace{-0.1cm}
    \caption{Qualitative results on YCB moving-object dataset. Performance is evaluated on video inputs and single frame inputs respectively. While segmentation looks similarly good in both cases, note that the single frame input results lose the ability to track objects, as indicated by the occasional change in object mask colourbetween frames.}
    \label{fig:seg_single_video}
\end{figure*}
\begin{table*}
    \centering
    \caption{The segmentation results on the YCB moving-object dataset evaluated on video inputs and single-frame inputs. The results are rounded to two decimal places. }
    \label{table:segmentation_single_video}
    \begin{adjustbox}{max width=1.0\textwidth}
    \begin{tabular}{l c c c}
        \hline
        & mIoU-BG$\uparrow$ & ARI-FG$\uparrow$ & MSC-FG$\uparrow$\\
        \midrule
        \textsc{\obpose~+ video inputs} & $1.00\pm0.00$ & $0.96\pm0.00$ & $0.97\pm0.00$ \\
        \textsc{\obpose~+ single frame inputs} & $1.00\pm0.00$ & $0.94\pm0.00$ & $0.97\pm0.00$ \\
        \bottomrule
    \end{tabular}
    \end{adjustbox}
\end{table*}

\subsection{More Qualitative Results}
We illustrate additional segmentation results on CLEVR-3D and MultiShapeNet datasets in \Cref{fig:seg_clevr_multi}.
\begin{figure*}[h]
    \centering
    \includegraphics[width=1.0\linewidth]{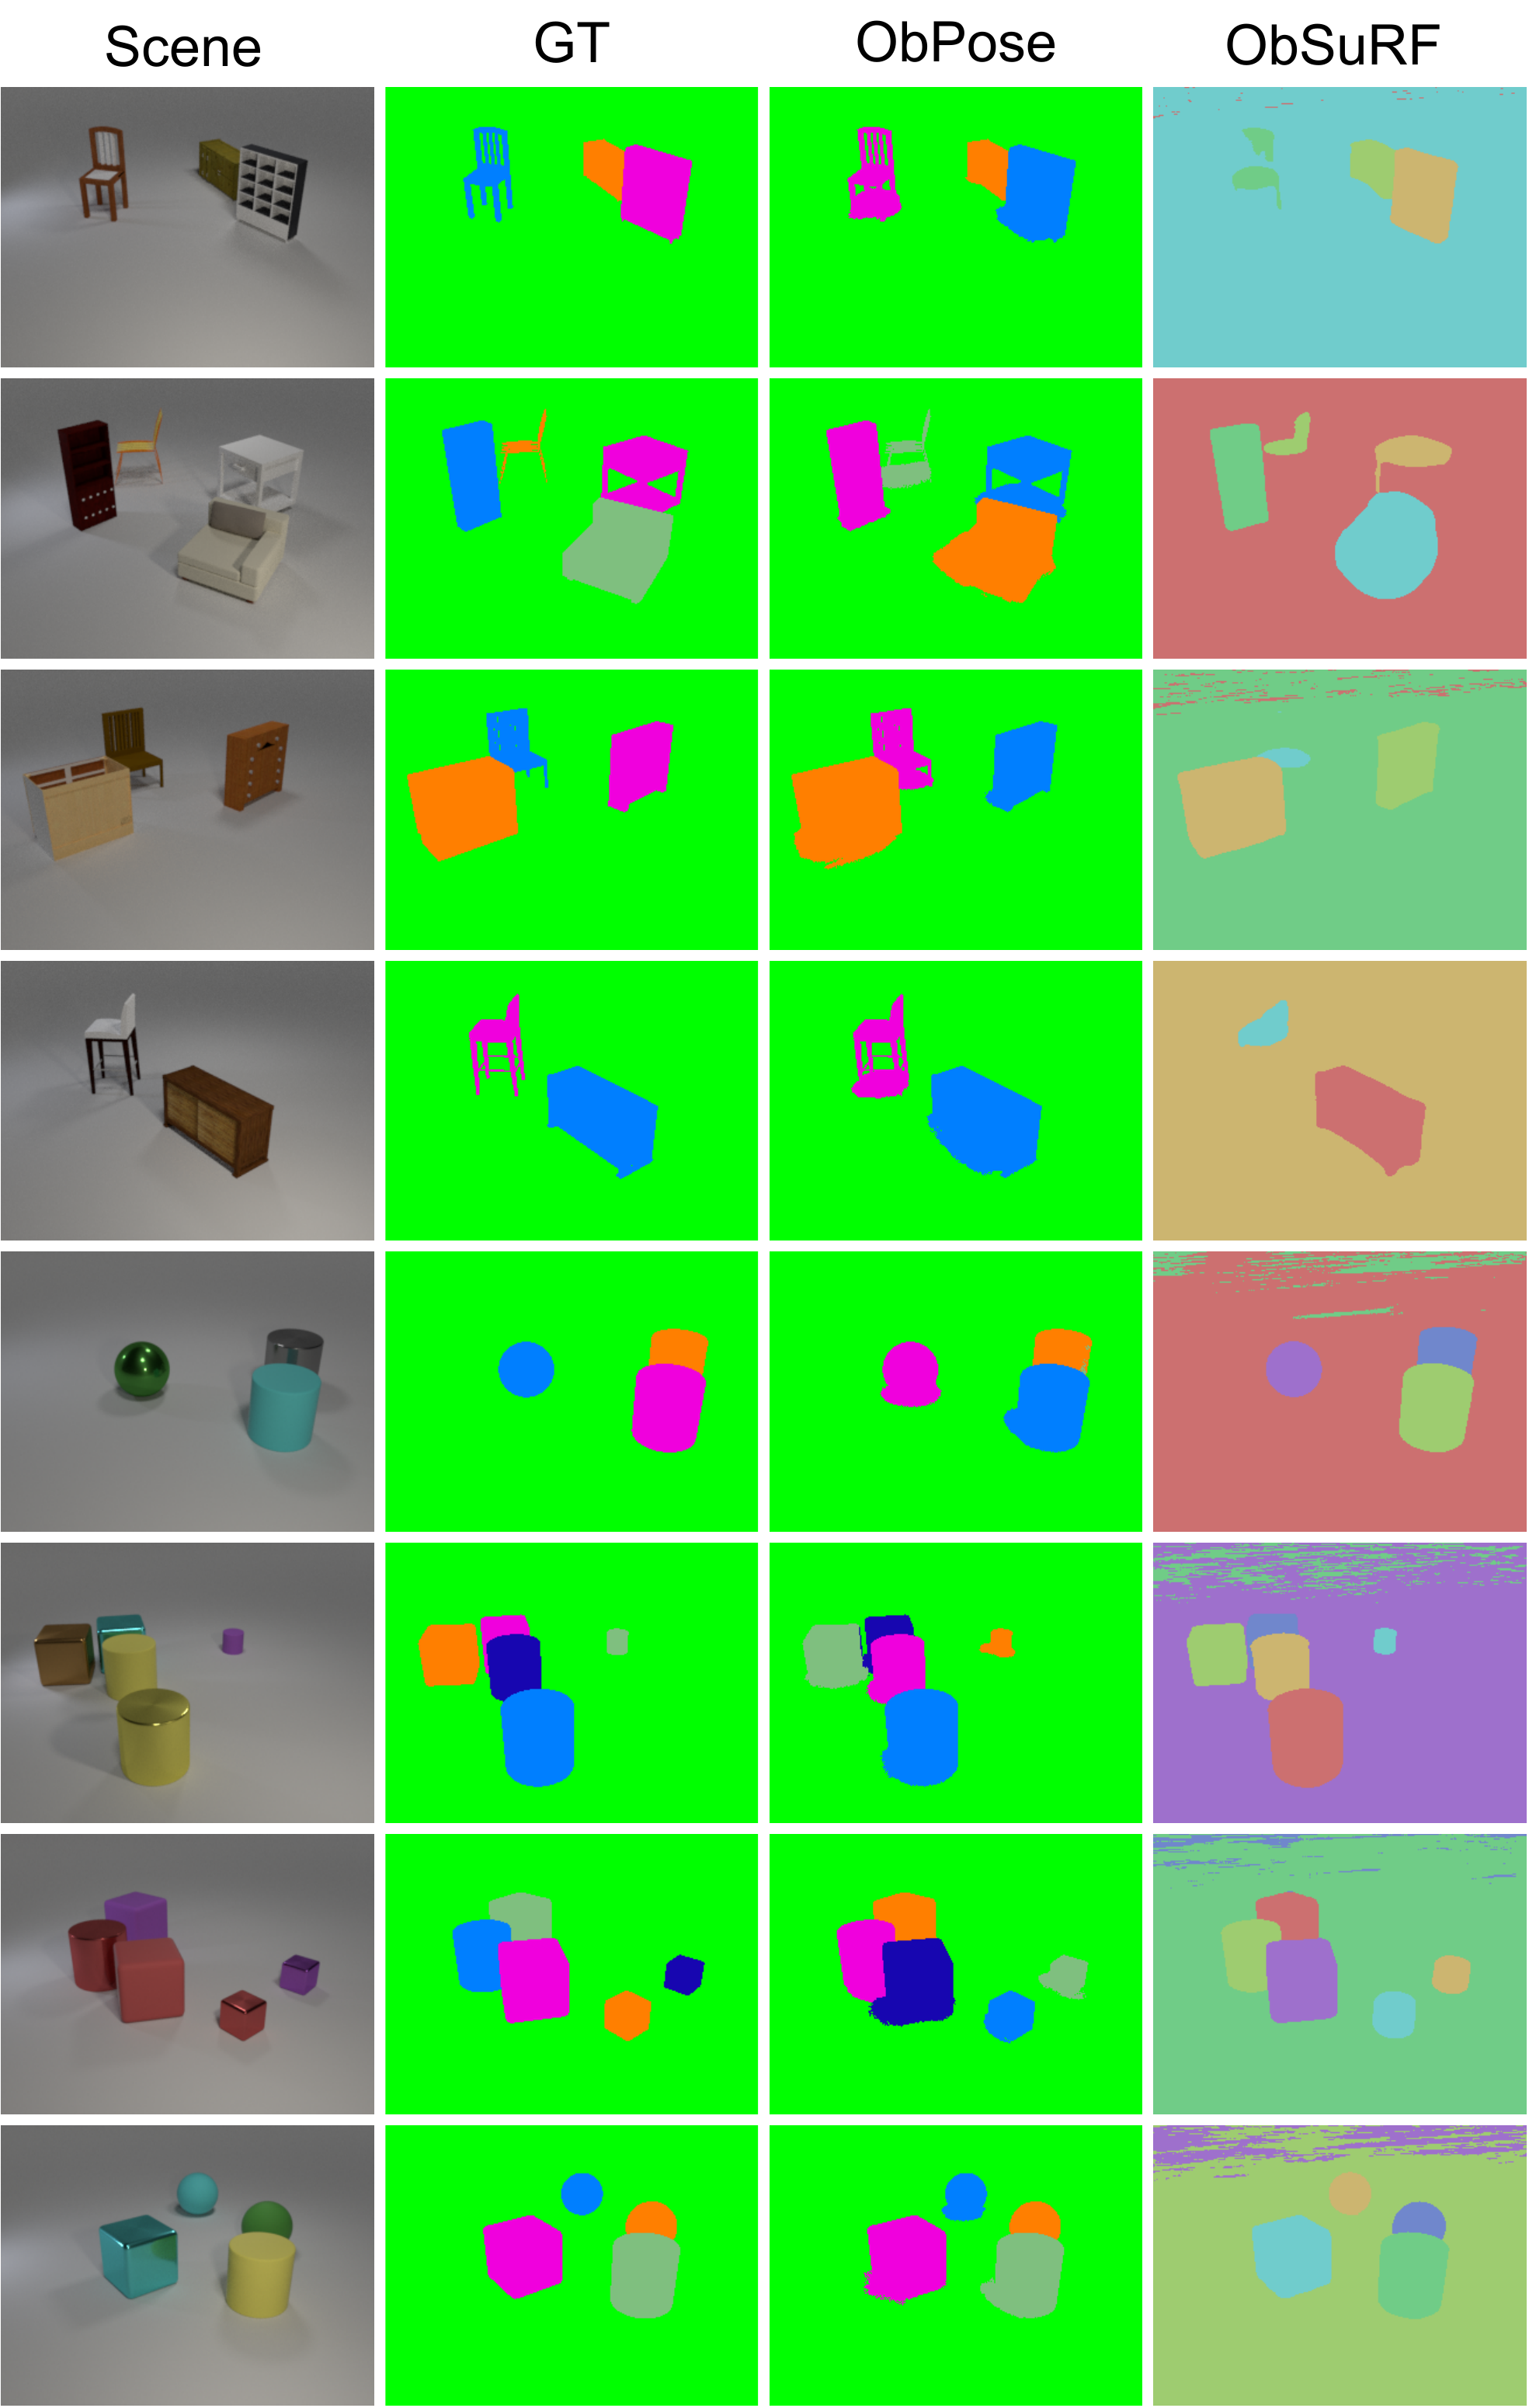}
    \vspace{-0.1cm}
    \caption{Qualitative results on CLEVR-3D and MultiShapeNet. We find that \obpose~can successfully identify part of the shadows of the objects. This is contradictory to the ground-truth labels where all object shadows are labelled as background.}
    \label{fig:seg_clevr_multi}
\end{figure*}
\subsection{Pose Estimation for Variance Reduction Encoding}
We show how the variance of the object appearance can be reduced by leveraging the shape-based estimated object location and orientation for the encoding of the objects in the \cref{fig:pose_new}.
\begin{figure*}[h]
    \centering
    \includegraphics[width=1.0\linewidth]{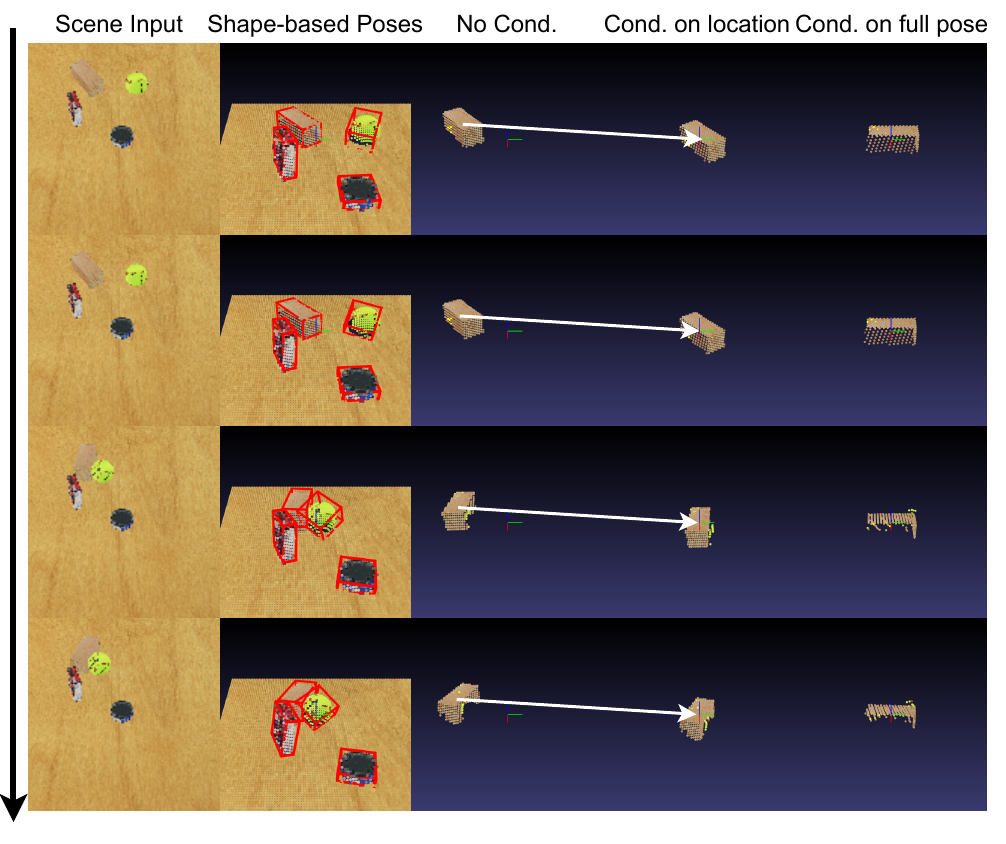}
    \vspace{-0.1cm}
    \caption{Visualisation of the recovered bounding boxes estimated from the object shape. We additionally illustrate the object (wooden box) appearance viewed by (a) being not conditioned on any location information (b) being conditioned on the shape-based estimated object location and (c) being conditioned on the shape-based estimated object location and orientation. We show that the variance of the object appearance is reduced leveraging the pose information.}
    \label{fig:pose_new}
\end{figure*}

\subsection{Limitations and Failure Mode}
The present work advances the state-of-the-art in unsupervised 3D-scene segmentation and interpretation. While \obpose~is important for advancing research, its impact outside of the machine learning community is low as current methods can not yet deal effectively with real images. This highlights the current limitations of the proposed model. In the future, we will investigate how to build a model that can explain complex real-world observations (e.g.~including shadows). \obpose~will then be ready for real-world robotics applications as a vision backbone.

An important failure mode of \obpose~is that our model can not predict meaningful object orientations when the object is severely occluded. In this case, we thus do not condition the encoding on the object orientation but only on the object location. Also, we found that the wooden box in the YCB static dataset is segmented as part of the background. We hypothesise that this is due to it having a similar texture to the wooden table (background). However, the wooden box is segmented correctly in the YCB video dataset, which would appear to suggest that the temporal structure of video can improve object segmentations.

%\subsection{Limitations and Potential Societal Impact}
%The present work advances the state-of-the-art in unsupervised 3D-scene segmentation and interpretation. While \obpose~is important for advancing research, its impact outside of the machine learning community is low as current methods can not yet deal effectively with real images. This highlights the current limitations of the proposed model. In the future, we will investigate how to build a model that can explain complex real-world observations including e.g.~shadows. \obpose~will then be ready for real-world robotics applications as a vision backbone.
